# Supplementary material for: Meta Clustering of Neural Bandits
Source: arXiv:2408.05586 source file (2024-09-27)
Supplement: Supplementary file 1 [file analysis4.tex]

\section{Another Form of Meta Generalization}

Here, we provide another version of Algorithm \ref{alg:meta} to update the meta-learner, as described in Algorithm \ref{alg:meta1}. Lemma \ref{lemma:metageneral} shows another generalization bound for the meta learner, which also can be thought of as a UCB for $\Theta$. However, compared to Lemma \ref{flemma:ucb}, Lemma \ref{lemma:metageneral} loses the information contained in meta gradients and user-side information. Therefore, we choose Lemma \ref{flemma:ucb} as the UCB of \sysn.

\begin{algorithm}[h]
\caption{SGD\_Meta ($\caln$) }\label{alg:meta1}
\begin{algorithmic}[1]
\State $\Theta_{(0)} =  \Theta_{0}$ (or  $\Theta_{t-1}$) \ \
\State $\calt^{\caln}_{t-1} = \emptyset$
\For{ $u \in \caln$}
\State Collect $ \mathcal{T}^{u}_{t-1}$ 
\State $\calt^{\caln}_{t-1} = \calt^{\caln}_{t-1} \cup  \mathcal{T}^{u}_{t-1}$
\EndFor
\For{$ j = 1, 2, \dots, | \calt^{\caln}_{t-1}| $}
\State Sequentially choose $ (\bx_j, r_j)  \in  \calt^{\caln}_{t-1} $ and corresponding $u_j$
\State $\call_j\left( \widehat{\theta}^{u_j}_{t-1}  \right) = \frac{1}{2} ( f(\bx_j;\widehat{\theta}^{u_j}_{t-1}) - r_j)^2  $
\State $\Theta_{(j)} = \Theta_{(j-1)} -  \eta_2 \triangledown_{\widehat{\theta}^{u_j}_{t-1}  }\call_j$
\EndFor
\State \textbf{Return:} Choose $\Theta_t$ uniformly from $\{\Theta_{(0)},  \dots, \Theta_{(| \calt^{\caln}|-1)}\}$ 
\end{algorithmic}
\end{algorithm}

\begin{lemma} \label{lemma:metageneral}
For any $\delta \in (0, 1), \rho \in (0, \calo(\frac{1}{L}))$, suppose $ 0<\epsilon_1, \epsilon_2  \leq 1$, and $m, \eta_1, \eta_2, J_1, J_2$ satisfy the conditions in Eq.(\ref{eq:conditions1}). Then with probability at least $1 -\delta$, for any $t \in [T]$, given a group $\caln$ and it's historical data $\calt^\caln_{t-1}$ where $\bar{t} = |\calt^\caln_{t-1}|$, it holds uniformly for Algorithm \ref{alg:meta1} that
\[
\underset{ \Theta_{t} \sim \{ \Theta_{(\tau-1)}\}_{\tau =1}^{\bar{t}}   }{\underset{(\bx, r) \sim \cald_u}{\underset{  (u, \cald_{u}) \sim \cald}{\bbe}}}\left[ |f(\bx; \Theta_{t}) - r|  | \calt^\caln_{t-1}  \right] \leq \sqrt{ \frac{2\epsilon_2}{\bar{t}}} + \frac{3L}{\sqrt{2\bar{t}}}  + (1+ \xi_2)\sqrt{\frac{ 2 \log(\calo(\bar{t}k)/\delta)}{\bar{t}}},
\]
where $\Theta_{t}$ is uniformly drawn from $\{ \Theta_{(\tau-1)}\}_{\tau =1}^{\bar{t}}$.
\end{lemma}

\begin{proof}
Let $\bar{t} = |\calt^\caln_{t-1}|$ and use $\{\bx_\tau, r_\tau\}_{\tau=1}^{\bar{t}}$ to represent $\calt^\caln_{t-1}$.

According to Lemma \ref{lemma:fthetabound2}, with probability at least $1 - \delta$, given any $\|\bx\|_2 = 1, r \leq 1$, for any $\tau \in [\bar{t}]$, we have
\begin{equation}
| f(\bx; \Theta_{(\tau)}) - r| \leq 1 + \xi_2.
\end{equation}
Then, define
\begin{equation}
V_\tau =  \underset{(\bx, r) \sim \cald_u}{\underset{  (u, \cald_{u}) \sim \cald}{\bbe}}\left[ |f(\bx; \Theta_{(\tau-1)}) - r| \right]  - | f(\bx_\tau; \Theta_{(\tau-1)})  - r_\tau|
\end{equation}
Then, we have
\begin{equation}
\bbe[V_{\tau} | \mathbf{F}_\tau] =    \underset{(\bx, r) \sim \cald_u}{\underset{  (u, \cald_{u}) \sim \cald}{\bbe}}\left[ |f(\bx; \Theta_{(\tau-1)}) - r| \right]  - \bbe \left[ | f(\bx_\tau; \Theta_{(\tau-1)})  - r_\tau| \right] = 0
\end{equation}
where $\mathbf{F}_\tau$ represents the $\sigma$-algebra generated by $\{\bx_{\tau'}, r_{\tau'} \}_{\tau' =1}^\tau$.
Therefore, according to Lemma 1 in \citep{cesa2004generalization}, applying Hoeffding-Azuma inequality to the bounded variables $V_1, \dots, V_t$, we have
\begin{equation}
\begin{aligned}
\frac{1}{\bar{t}} \sum_{\tau = 1}^{\bar{t}}  \underset{(\bx, r) \sim \cald_u}{\underset{  (u, \cald_{u}) \sim \cald}{\bbe}}\left[ |f(\bx; \Theta_{(\tau-1)}) - r| \right]  
\leq  \frac{1}{\bar{t}}\sum_{\tau = 1}^{\bar{t}} | f(\bx_\tau; \Theta_{(\tau-1)})  - r_\tau| + (1+ \xi_2)\sqrt{\frac{ 2 \log(1/\delta)}{\bar{t}}}.
\end{aligned}
\end{equation}
Accoding to Algorithm \ref{alg:meta1}, we have
\begin{equation}
 \underset{ \Theta_{t} \sim \{ \Theta_{(\tau-1)}\}_{\tau=1}^{\bar{t}}   }{\underset{(\bx, r) \sim \cald_u}{\underset{  (u, \cald_{u}) \sim \cald}{\bbe}}}\left[ |f(\bx; \Theta_{t}) - r| \right]   =  \frac{1}{\bar{t}} \sum_{\tau = 1}^{\bar{t}}  \underset{(\bx, r) \sim \cald_u}{\underset{  (u, \cald_{u}) \sim \cald}{\bbe}}\left[ |f(\bx;  \Theta_{(\tau-1)}) - r| \right]  
\end{equation}
Therefore, we have
\begin{equation} \label{eq:g1}
\underset{ \Theta_{t} \sim \{ \Theta_{(\tau-1)}\}_{\tau =1}^{\bar{t}}   }{\underset{(\bx, r) \sim \cald_u}{\underset{  (u, \cald_{u}) \sim \cald}{\bbe}}}\left[ |f(\bx; \Theta_{t}) - r| \right] \leq  \underbrace{ \frac{1}{\bar{t}}\sum_{\tau = 1}^{\bar{t}} | f(\bx_\tau; \Theta_{(\tau-1)})  - r_\tau|}_{I_1} + (1+ \xi_2)\sqrt{\frac{ 2 \log(1/\delta)}{ \bar{t}}}.
\end{equation}
For $I_1$, Applying the Lemma \ref{lemma:caogenelimetab}, for any $\Theta' \in \bbr^p$ satisfying $\|\Theta' - \Theta_0\|_2 \leq \beta_2$, we have
\begin{equation} \label{eq:g2}
\frac{1}{\bar{t}}\sum_{\tau = 1}^{\bar{t}} | f(\bx_\tau; \Theta_{(\tau-1)})  - r_\tau| \leq \underbrace{ \frac{1}{\bar{t}}\sum_{\tau = 1}^{\bar{t}}  | f(\bx_\tau; \Theta')  - r_\tau| }_{I_2} + \frac{3L}{\sqrt{2 \bar{t}}}
\end{equation}
For $I_2$, we have
\begin{equation}\label{eq:g3}
\frac{1}{\bar{t}}\sum_{\tau = 1}^{\bar{t}}  | f(\bx_\tau; \Theta')  - r_\tau| \leq \frac{1}{\bar{t}}\sqrt{\bar{t}} \sqrt{  \sum_{\tau = 1}^{\bar{t}}  ( f(\bx_\tau; \Theta')  - r_\tau)^2}
\leq \frac{1}{\sqrt{\bar{t}}} \sqrt{2\epsilon_2}.
\end{equation}
where the last inequality is according to \ref{lemma:thetaconvergence2}: there exists $ \Theta'$ satisfying  $ \| \Theta' - \Theta_0\|_2 \leq \beta_2 $, such that $\frac{1}{2} \sum_{\tau=1}^{\bar{t}} ( f(\bx_\tau; \Theta') - r_\tau)^2 \leq \epsilon_2$.

In the end, combining Eq.(\ref{eq:g1}), Eq.(\ref{eq:g2}), and Eq.(\ref{eq:g3}), we have
\begin{equation}
\underset{ \Theta_{t} \sim \{ \Theta_{(\tau-1)}\}_{\tau =1}^{\bar{t}}   }{\underset{(\bx, r) \sim \cald_u}{\underset{  (u, \cald_{u}) \sim \cald}{\bbe}}}\left[ |f(\bx; \Theta_{\tau}) - r| \right] \leq \sqrt{ \frac{2\epsilon_2}{\bar{t}}} + \frac{3L}{\sqrt{2 \bar{t}}}  + (1+ \xi_2)\sqrt{\frac{ 2 \log(1/\delta)}{\bar{t}}}.
\end{equation}
Apply the union bound for $\tau \in [\bar{t}], i \in [k]$ and the proof is completed.
\end{proof}

\begin{lemma}\label{lemma:fthetabound2}
For any $\delta \in (0, 1), \rho \in (0, \calo(\frac{1}{L}))$, $0 < \epsilon_1 \leq \epsilon_2 < 0, \lambda > 0$, suppose $m, \eta_1, \eta_2, J_1, J_2$ satisfy the conditions in Eq.(\ref{eq:conditions1}). Then, with probability at least $1-\delta$, for any $j \in [\bar{t}]$ we have
\[
| f(\bx; \Theta_{(j)})| \leq \left( 2 +  \calo(L\beta_2) + \mathcal{O}((L+1)^2 \sqrt{m \log m} \beta_2^{4/3})\right) = \xi_2
\]

\end{lemma}

\begin{proof}
Based on Lemma \ref{lemma:wanggenef}, 
Then, we have
\begin{equation}
\begin{aligned}
\Rightarrow  
 | f(\bx; \Theta_{(j)})  |   \leq    & \underbrace{| f(\bx; \Theta_0)  |}_{I_1} +  \underbrace{ |  \langle \triangledown_{\Theta}f(\bx; \Theta_{0}),   \Theta_{(j)} - \Theta_{0} \rangle |}_{I_2} +     \mathcal{O}(w^{1/3}(L+1)^2 \sqrt{m \log m}) \| \Theta_{(j)} - \Theta_{0}  \|_2 \\
\leq  & \underbrace{ 2\|\bx\|_2}_{I_1} + \underbrace{ \|\triangledown_{\Theta}f(\bx; \Theta_{0})\|_2 \|   \Theta_{(j)} - \Theta_{0}   \|_2}_{I_2}  + \mathcal{O}(w^{1/3}(L+1)^2 \sqrt{m \log m}) \| \Theta_{(j)} - \Theta_{0}  \|_2 \\ 
\underbrace{\leq}_{E_3} & 2  + \calo(L) \cdot \beta_2 +  \mathcal{O}((L+1)^2 \sqrt{m \log m})\beta_2^{4/3}
\end{aligned}
\end{equation}
where $I_1$ is the applying of Lemma 7.3 in \citep{allen2019convergence}, $I_2$ is by Cauchy–Schwarz inequality, and $E_3$ is due to Lemma \ref{lemma:thetaconvergence2}.
\end{proof}

\begin{lemma}[\citep{wang2020globalcon}] \label{lemma:wanggenef}
Suppose $m$ satisfies the condition2 in  Eq.(\ref{eq:conditions1}), if
\[
     \Omega( m^{-3/2}L^{-3/2} [\log (TkL^2/\delta)]^{3/2} ) \leq \nu \leq \mathcal{O}((L+1)^{-6}\sqrt{m}).
\]
then with probability at least $1 - \delta$, for all $\Theta, \Theta'$ satisfying $\| \Theta - \Theta_0\|_2 \leq \nu$ and $\|\Theta' - \Theta_0\|_2 \leq \nu$, $\bx \in \bbr^d$,  $\|\bx\|_2 = 1$,  we have
\[
|f(\bx; \Theta) - f(\bx; \Theta') - \langle \triangledown_{\Theta}f(\bx; \Theta),   \Theta' - \Theta \rangle| \leq \mathcal{O}( \nu^{4/3} (L+1)^2 \sqrt{m \log m} ).
\]
\end{lemma}

\begin{lemma} \label{lemma:caogenelimetab}
For any $\delta \in (0, 1)$, suppose
\[
m > \tilde{\mathcal{O}}\left(  \text{poly} (T, n, \delta^{-1}, L) \cdot  \log (1/\delta) \cdot e^{\sqrt{ \log 1/\delta}} \right), \ \ \nu = \boldsymbol{\Theta}(\bar{t}^6/\delta^2).  
\]
Then, with probability at least $1 - \delta$, set $\eta_2 =  \Theta( \frac{ \nu}{\sqrt{2} \bar{t} m})$, for any $\Theta' \in \bbr^p$ satisfying $\|\Theta' - \Theta_0\|_2 \leq \beta_2$ ,  such that
\[
\begin{aligned}
 \sum_{\tau=1}^{\bar{t}} | f(\bx_{\tau}; \Theta_{(j)} - r_\tau|  & \leq \sum_{\tau =1 }^{\bar{t}} | f(\bx_{\tau}; \Theta') - r_\tau| + \frac{3L\sqrt{ \bar{t}} }{\sqrt{2}} \\
\end{aligned}
\]
\end{lemma}
\begin{proof}
Then, the proof is a direct application of Lemma 4.3 in \citep{cao2019generalization} by setting the loss as $L_\tau(\widehat{\Theta}_{\tau}) = | f(\bx_{\tau}; \widehat{\Theta}_{\tau}) - r_\tau|  $, $R = \beta_2 \sqrt{m} ,  \epsilon = \frac{LR}{ \sqrt{2\nu \bar{t}}}$,  and $ \nu = R^2$.

\end{proof}
