# Supplementary material for: Meta Clustering of Neural Bandits
Source: arXiv:2408.05586 source file (2024-09-27)
Supplement: Supplementary file 2 [file appendix_new.tex]

\section{Proof Details of Theorem \ref{theorem:main}} \label{sec:proofs}

Our proof technique is different from related works. \citep{2014onlinecluster,2016collaborative,gentile2017context,2019improved,ban2021local} are built on the classic linear bandit framework and \citep{zhou2020neural, zhang2020neural, kassraie2022neural} utilize the kernel-based analysis in the NTK regime. 
%We directly upper bound the mean of regret of overall $T$ rounds by  
In contrast, we use the generalization bound of user-learner to bound the error incurred in each round and bridge meta-learner with user-learner by bounding their distance, which leads to our final regret bound.
Specifically, we decompose the regret of $T$ rounds into three key terms, where the first term is the error induced by user learner $\theta^u $, the second term is the distance between user learner and meta learner, and the third term is the error induced by the meta learner $\Theta$. 
Then, Lemma \ref{lemma:userboundasttheta} provides an upper bound for the first term. Lemma \ref{lemma:userboundasttheta} is an extension of Lemma \ref{lemma:genesingle}, which is the key to removing the input dimension. Lemma \ref{lemma:genesingle} has two terms with the complexity $\calo(\sqrt{T})$, where the first term is the training error induced by a class of functions around initialization, the second term is the deviation induced by concentration inequality for $f(\cdot; \theta^u)$. Lemma \ref{lemma:metauserdistance} bounds the distance between user-learner and meta-learner. 
Lemma \ref{lemma:ucb} bounds the error induced by the meta learner using triangle inequality bridged by the user learner.
Bounding these three terms completes the proof.

%We first show the lemmas for the analysis of user-learner in Section \ref{proof:banditlearner}, the lemmas for meta-learner in Section \ref{proof:metalearner}, the lemma to bridge bandit-learner and meta-learner in Section \ref{proof:bridge}, and the lemmas for the main workflow in Section \ref{sec:mainproof}.

\subsection{Analysis for user-learner}\label{proof:banditlearner}

Following \cite{allen2019convergence, cao2019generalization}, given an instance $\bx \in \bbe^d$ with $\|\bx\|_2 = 1$, we define the outputs of hidden layers of the neural network (Eq. (\ref{eq:structure})):
\[
\bh_0 = \bx,  \bh_l = \sigma(\bw_l \bh_{l-1}), l \in [L-1].
\]
Then, we define the binary diagonal matrix functioning as ReLU:
\[
\bD_l = \text{diag}( \mathbbm{1}\{(\bw_l \bh_{l-1})_1 \}, \dots, \mathbbm{1}\{(\bw_l \bh_{l-1})_m \} ), l \in [L-1].
\]
Accordingly, given an input $\bx$, the neural network (Eq. (\ref{eq:structure})) is represented by 
\[
f(\bx_t; \theta \ \text{or} \ \Theta) = \bw_L (\prod_{l=1}^{L-1} \bD_l \bw_l) \bx,
\]
and
\[
\nabla_{\bw_l}f  = 
\begin{cases}
[\bh_{l-1}\bw_L (\prod_{\tau=l+1}^{L-1} \bD_\tau \bw_\tau)]^\top, l \in [L-1] \\
\bh_{L-1}^\top,   l = L .
\end{cases}
\]
Given a reward $r \in [0, 1]$, define $\call(\theta) = (f(\bx; \theta) - r)^2/2$.
Then, we have the following auxiliary lemmas.

\begin{lemma} \label{lemma:xi1}
 Suppose $m, \eta_1, \eta_2$ satisfy the conditions in Theorem \ref{theorem:main}.  With probability at least $1 -  \calo(TKL)\cdot \exp(-\Omega(m \omega^{2/3}L))$ over the random initialization, for all $t \in [T], i \in [k] $,  $\theta$ (or $\Theta$) satisfying $ \|\theta - \theta_0\|_2 \leq \omega$ with $ \omega \leq \calo(L^{-9/2} [\log m]^{-3})$, it holds uniformly that
\[
\begin{aligned}
&(1), | f(\bx; \theta)| \leq  \calo(1). \\
&(2), \| \nabla_{\theta}    f(\bx; \theta) \|_2 \leq \calo(\sqrt{L}). \\
&(3), \|  \nabla_{\theta} \call(\theta)  \|_2 \leq  \calo(\sqrt{L})
\end{aligned}
\]
\end{lemma}

\begin{lemma} \label{lemma:functionntkbound}
Suppose $m, \eta_1, \eta_2$ satisfy the conditions in Theorem \ref{theorem:main}.  With probability at least $1 -  \calo(TKL)\cdot \exp(-\Omega(m \omega^{2/3}L))$, for all $t \in [T], i \in [k] $, $\theta, \theta'$ (or $\Theta, \Theta'$ ) satisfying $ \|\theta - \theta_0\|_2,  \|\theta' - \theta_0\|_2 \leq \omega$ with $ \omega \leq \calo(L^{-9/2} [\log m]^{-3})$, it holds uniformly that
\[
| f(\bx; \theta) - f(\bx; \theta') -  \langle  \triangledown_{\theta'} f(\bx; \theta'), \theta - \theta'    \rangle    | \leq \mathcal{O} (\omega^{1/3}L^2 \sqrt{ \log m}) \|\theta - \theta'\|_2.
\]
\end{lemma}

\begin{lemma}  \label{lemma:differenceee}
Suppose $m, \eta_1, \eta_2$ satisfy the conditions in Theorem \ref{theorem:main}.  With probability at least $1 -  \calo(TKL)\cdot \exp(-\Omega(m \omega^{2/3}L))$, for all $t \in [T], i \in [k] $,  $\theta, \theta'$ satisfying $ \|\theta - \theta_0\|_2,  \|\theta' - \theta_0\|_2 \leq \omega$ with $ \omega \leq \calo(L^{-9/2} [\log m]^{-3})$, it holds uniformly that
\begin{equation}
\begin{aligned}
 (1) \qquad  & |f(\bx; \theta) - f(\bx; \theta')|  \leq   \calo(  \omega \sqrt{L})  +  \mathcal{O} (\omega^{4/3}L^2 \sqrt{ \log m})
 \end{aligned}
\end{equation}
\end{lemma}

\begin{lemma} [Almost Convexity]  \label{lemma:convexityofloss} 
Let $\call_t(\theta) = (f(\bx_t; \theta) - r_t)^2/2 $.  Suppose $m, \eta_1, \eta_2$ satisfy the conditions in Theorem \ref{theorem:main}.  For any $\epsilon > 0$,  with probability at least $1- \calo(TKL^2)\exp[-\Omega(m \omega^{2/3} L)] $ over randomness of $\theta_1$, for all $ t \in [T]$, and $\theta, \theta'$
satisfying $\| \theta - \theta_0 \|_2 \leq \omega$ and $\| \theta' - \theta_0 \|_2 \leq \omega$ with $\omega \leq \calo(L^{-6} [\log m]^{-3/2} \epsilon^{3/4})$, it holds uniformly that
\[
 \call_t(\theta')  \geq  \call_t(\theta) + \langle \nabla_{\theta}\call_t(\theta),      \theta' -  \theta     \rangle  -  \epsilon.
\]
\end{lemma}

\begin{lemma}[User Trajectory Ball] \label{lemma:usertrajectoryball}
Suppose $m, \eta_1, \eta_2$ satisfy the conditions in Theorem \ref{theorem:main}. 
With probability at least $1- \calo(TKL^2)$
$\exp[-\Omega(m \omega^{2/3} L)] $ over randomness of $\theta_0$, for any $R > 0$, it holds uniformly that
\[
\|\theta_t - \theta_0\|_2 \leq \calo(R/m^{1/4}) \leq \calo(L^{-6} [\log m]^{-3/2} T^{-3/4}), t \in [T].
\]
\end{lemma}

\begin{lemma} [Instance-dependent Loss Bound] \label{lemma:instancelossbound}
Let $\call_t(\theta) = (f(\bx_t; \theta) - r_t)^2/2$. 
 Suppose $m, \eta_1, \eta_2$ satisfy the conditions in Theorem \ref{theorem:main}. 
With probability at least $1- \calo(TKL^2)\exp[-\Omega(m \omega^{2/3} L)] $ over randomness of $\theta_0$, given any $R > 0$  it holds that
\begin{equation}
\sum_{t=1}^T \call_t(\theta_t)  \leq  \sum_{t=1}^T  \call_t(\theta^\ast) +  \calo(1) +  \frac{TLR^2}{\sqrt{m}}.
\end{equation}
where $\theta^\ast =  \arg \inf_{\theta' \in B(\theta_0, R)}  \sum_{t=1}^T  \call_t(\theta')$.
\end{lemma}

\begin{lemma} \label{lemma:genesingle}
For any $\delta \in (0, 1),  R > 0 $, and $m , \eta_1, \eta_2$ satisfy the conditions in Theorem \ref{theorem:main}. In a round $\tau$ where $u \in N$ is serving user, let $x_\tau$ be the selected arm and $r_\tau$ is the corresponding received reward.
Then, with probability at least $1 -\delta$ over the randomness of initialization, the cumulative regret induced by $u$ up to round $T$ is upper bounded by:
\[
\begin{aligned}
 & \frac{1}{\mu_T^u} \sum_{ (\bx_\tau, r_\tau ) \in \calt_{T}^u }  \underset{r_\tau | \bx_\tau}{\bbe} [ |f(\bx_\tau; \theta^u_{\tau-1}) - r_\tau|] \\
\leq &  \sqrt{ \frac{S^{\ast}_T(u) + \calo(1) }{\mu_T^u}} + \calo \left(\sqrt{\frac{2 \log( \calo (1) /\delta)}{\mu^u_T}} \right) .
\end{aligned}
\]
where $S^{\ast}_T(u) = \underset{\theta \in B(\theta_0, R)}{\inf} \sum_{ (\bx_\tau, r_\tau) \in  \calt_{T}^u} L_\tau(\theta)$.
\end{lemma}

\begin{lemma} \label{lemma:utroundsregret}
For any $\delta \in (0, 1),  R > 0 $, and $m , \eta_1, \eta_2$ satisfy the conditions in Theorem \ref{theorem:main}.
Suppose $ \widehat{\caln}_{u_t}(\bx_t) =  \caln_{u_t}(\bx_t), \forall t \in [T]$.
After $T$ rounds, with probability $1-\delta$ over the random initialization, the cumulative error induced by the bandit-learners is upper bounded by
\[
\begin{aligned}
& \sum_{t=1}^T  \frac{1}{|\caln_{u_t}(\bx_t) |} \sum_{u_{t,i}  \in \caln_{u_t}(\bx_t) }   \underset{  r_t | \bx_t }{\bbe} [ |f(\bx_t; \theta^{u_{t,i}}_{t-1}) - r_t| ] \\
\leq &  \sqrt{ q T \cdot S^{\ast}_{Tk}  \log(\calo (\delta^{-1}))  + \calo(1) }    + \calo(\sqrt{     2 q T \log(\calo (\delta^{-1}))}) ,
\end{aligned}
\]
where  $S^{\ast}_{Tk} = \underset{\theta \in B(\theta_0, R)}{\inf} \sum_{t=1}^{Tk}\call_{t}(\theta)$ .
\end{lemma}

\begin{corollary} \label{lemma:genesingleast}
For any $\delta \in (0, 1),  R > 0 $, and $m , \eta_1, \eta_2$ satisfy the conditions in Theorem \ref{theorem:main}.
In a round $\tau$ where $u \in N$ is the serving user, let $x_\tau^\ast$ be the arm selected according to Bayes-optimal policy $\pi^\ast$: 
\[
x_\tau^\ast = \arg \max_{\bx_{\tau,i}, i \in [k]} h_{u} (\bx_{\tau, i}),  
\]
and $r_\tau^\ast$ is the corresponding reward.
Then, with probability at least $1 -\delta$ over the randomness of initialization, after $t \in [T]$ rounds, the cumulative regret induced by $u$ with policy $\pi^\ast$ is upper bounded by: 
\[
\begin{aligned}
 &        \frac{1}{\mu_t^u} \sum_{ (\bx_\tau^\ast, r_\tau^\ast ) \in \calt_{t}^{u, \ast} }     \underset{  r_\tau^\ast | \bx_\tau^\ast  }{\bbe}  [ |f(\bx_\tau^\ast; \theta^{u, \ast}_{\tau-1}) - r_\tau^\ast| \mid \pi^\ast]  \\
\leq &   \sqrt{ \frac{ S^{\ast}_T (u) + \calo(1) }{\mu_t^u}} + \calo \left(\sqrt{\frac{2 \log( \calo (1) /\delta)}{\mu^u_t}} \right) .
\end{aligned}
\]
where  $S^{\ast}_T (u) = \underset{\theta \in B(\theta_0, R)}{\inf} \sum_{ (\bx_\tau^\ast, r_\tau^\ast) \in  \calt_{t}^{u, \ast}} L_\tau(\theta)$, and $\calt_{t}^{u, \ast} $ are stored Bayes-optimal pairs up to round $t$ for $u$, and $\theta^{u, \ast}_{\tau-1}$ are the parameters trained on  $\calt_{\tau-1}^{u, \ast}$ according to SGD\_User in round $\tau-1$.
\end{corollary}

\begin{corollary} \label{lemma:userboundasttheta}
For any $\delta \in (0, 1),  R > 0 $, and $m , \eta_1, \eta_2$ satisfy the conditions in Theorem \ref{theorem:main}.
In round $t \in [T]$, given $u \in N$,
let 
\[
x_t^\ast = \arg \max_{\bx_{t,i}, i \in [k]} h_{u} (\bx_{t, i})  
\]
the  Bayes-optimal arm for $u$ and $r_t^\ast$ is the corresponding reward.
Then, with probability at least $1 -\delta$ over the random initialization, after $T$ rounds, with probability $1-\delta$ over the random initialization, the cumulative error induced by the bandit-learners is upper bounded by:
\[
\begin{aligned}
& \sum_{t=1}^T \underset{  r_t^\ast \mid \bx_t^\ast }{\bbe} [ |f(\bx_t^\ast; \theta^{u_t, \ast}_{t-1}) - r_t^\ast|] \\
\leq &  \sqrt{  q T \cdot S^{\ast}_{Tk}  + \calo(1) }    + \calo(\sqrt{   2 qT \log(\calo (1) /\delta)}).
\end{aligned}
\]
where  the expectation is taken over $r_\tau^\ast$ conditioned on $\bx_\tau^\ast$ and $\theta^{u_t, \ast}_{t-1}$ are the parameters trained on  $\calt_{t-1}^{u_t, \ast}$ according to SGD in round $t-1$.
\end{corollary}

\subsection{ Bridge Meta-learner and User-learner} \label{proof:bridge}

For brevity, we use $ g(\bx_t; \theta_{t-1}^{u})$ to represent the gradient $\nabla_{\theta} f(\bx_t; \theta_{t-1}^{u})$.

\begin{lemma}  \label{lemma:metauserdistance}
Suppose $m, \eta_1, \eta_2$ satisfy the conditions in Theorem \ref{theorem:main}. 
With probability at least $1- \calo(nTKL^2)\exp[-\Omega(m \omega^{2/3} L)] $ over randomness of $\Theta_0$, for all $t \in [T]$, 
any $u \in N$ and $\Theta_t$ returned by Algorithm \ref{alg:meta}, for any $\|\bx_t\|_2 = 1$, it holds uniformly for Algorithms \ref{alg:main}-\ref{alg:meta} that
\begin{equation}
\begin{aligned}
| f(\bx_t; \theta_{t-1}^{u}) -  f(\bx_t; \Theta_{t}) |   \leq 
\frac{R\| \nabla_{\Theta} f(\bx_t; \Theta_{t}) - \nabla_{\theta} f(\bx_t; \theta_{0}^{u})\|_2}{m^{1/4}}  + Z,
\end{aligned}
\end{equation}
where 
\[
Z  =   \frac{\mathcal{O} (RL^2 \sqrt{\log m} ) }{m^{1/3}} +      \frac{\calo ( L^{7/3}R^2  \sqrt{\log m})}{m^{1/2}}  +  \frac{\mathcal{O}(2 R \sqrt{L}) }{ m^{1/4}}. \\ 
\]
\end{lemma}

\begin{lemma} \label{lemma:ucb}
Suppose $m, \eta_1, \eta_2$ satisfy the conditions in Theorem \ref{theorem:main}. Then, with probability at least $1- \delta$ over the random initialization, for any $\delta \in (0, 1), R> 0$, after $t$ rounds, the error induced by meta-learner is upper bounded by:
\begin{equation}
\begin{aligned}
&    \sum_{t=1}^T  \underset{ r_t \mid \bx_t}{\bbe} \left[ |f(\bx_{t}; \Theta_{t}) - r_{t}|  \mid u_t \right] \\
\leq &
     \sum_{t=1}^T   \frac{R\| g(\bx_t; \Theta_{t}) - g(\bx_t; \theta_{0}^{u_t})\|_2}{m^{1/4}} + 
  \sum_{u \in N}  \mu_T^{u}   \Bigg  [  \calo \left( \frac{\sqrt{S^{\ast}_{Tk}  + \calo(1) } }{\sqrt{2\mu^{u}_{T}}}  \right) \\
&  +   \sqrt{\frac{  2 \log(  \calo(1) /\delta) }{\mu^{u}_T}} \Bigg].
\end{aligned}
\end{equation}
where the expectation is taken over $r_t$ conditioned on $x_t$.
\end{lemma}

\section{Connections with Neural Tangent Kernel}

\begin{lemma} [Lemma \ref{lemma:upperboundofStk} Restated]
Suppose $m$ satisfies the conditions in Theorem \ref{theorem:main}. With probability at least $1 - \delta$ over the initialization, there exists $\btheta'  \in  B(\theta_0, \widetilde{\Omega}(T^{3/2}))$, such that
\[
\begin{aligned}
\bbe[S^{\ast}_{Tk}] & \leq    \sum_{t=1}^{TK} \bbe [ ( r_t -  f(\bx_t; \theta'))^2/2 ]  \\
&\leq \calo \left(\sqrt{ \widetilde{d} \log(1 + TK) - 2 \log \delta  } + S + 1 \right)^2 \cdot \widetilde{d} \log (1+TK).
\end{aligned}
\]
\end{lemma}

\iffalse
\begin{definition} \label{def:ridge}
Given the context vectors $\{\bx_i\}_{i=1}^T$ and the rewards $\{ r_i \}_{i=1}^{T} $, then we define the estimation $\widehat{\theta}_t$ via ridge regression:  
\[
\begin{aligned}
&\mathbf{A}_t = \mathbf{I} + \sum_{i=1}^{t} g(\bx_i; \theta_0) g(\bx_i; \theta_0)^\top \\
&\mathbf{b}_t = \sum_{i=1}^{t} r_i g(\bx_i; \theta_0)  \\
&\widehat{\theta}_t = \mathbf{A}^{-1}_t \mathbf{b}_t 
\end{aligned}
\]
\end{definition}
\fi

\begin{lemma}\label{lemma:bounfofsinglethetaprime}
Suppose $m$ satisfies the conditions in Theorem \ref{theorem:main}. With probability at least $1 - \delta$ over the initialization, there exists $\btheta'  \in  B(\theta_0, \widetilde{\Omega}(T^{3/2}))$ for all $t \in [T]$, such that
\[
\begin{aligned}
     & | \hx  - f(\bx_t; \theta') |  \\
\leq  & \calo \left ( \sqrt{  \log \left(  \frac{\deter(\mathbf{A}_t)} { \deter(\mathbf{I}) }   \right)   - 2 \log  \delta }  +  S  + 1  \right) \| \gx  \|_{\mathbf{A}_{t}^{-1}} \\
&+ \calo \left(\frac{T^2 L^3 \sqrt{\log m}}{m^{1/3}} \right)
\end{aligned}
\]
\end{lemma}

\subsection{Additional Results} \label{sec:additionalresults}

\textit{Convergence rate on MovieLens and Yelp}.
Table \ref{tab:convergencerate} illustrates the average cumulative regrets of \sysn for different time step intervals of 2000 rounds on the MovieLens and Yelp datasets. It's noticeable that the average regret per round of \sysn decreases as more time steps are considered.
One plausible explanation for the "linear-like" curves in the cumulative regrets is that both the MovieLens and Yelp datasets used for recommendation tasks contain inherent noise. This noise can make it challenging for algorithms to accurately learn the underlying reward mapping function. Consequently, achieving substantial experimental improvements on these datasets can be quite challenging.
In essence, the presence of noise in the data can lead to fluctuations in the regret curves, making it appear as if progress is linear rather than exponential or logarithmic. Despite these challenges, the algorithm, \sysn, continues to make progress in minimizing regret over time.

\begin{table}[ht]
	\vspace{1em}
	\centering
	\begin{tabular}{c|c|c|c|c|c}
		\toprule 
 Rounds   &   2000 & 4000 & 6000 & 8000 & 10000   \\ 
	\toprule  
MovieLens & 0.4717 & 0.4555  & 0.4475  & 0.4452  & 0.4442\\
Yelp & 0.7532 & 0.7395 & 0.7358 & 0.7306 & 0.7269 \\
\bottomrule
	\end{tabular}
 	\caption{  Convergence rate of \sysn on MovieLens and Yelp }\label{tab:convergencerate}
\end{table}

\iffalse
\textit{Ablation Study for Input Dimension}. We run the experiments on MovieLens dataset with different input dimensions and report the results as follows. Table \ref{tabinput} summarizes the final regret of each method with different input dimensions (5 runs). \sysn keeps the similar regret with the small fluctuation. This fluctuation is acceptable given that different input dimensions may contain different amount of information. NeuUCB-ONE and NeuUCB-IND also use the neural network to learn the reward function, so they have the similar property. In contrast, the regret of linear bandits (CLUB, COFIBA, SCLUB, LOCB) is affected more drastically by the input dimensions, which complies with their regret analysis.

\fi

\begin{table}[ht]
\centering
\begin{tabular}{c|cccccc|c}
\hline
               & NeuUCB-ONE         & NeuUCB-IND     & \sysn      \\ \hline
2 layers            & 4839.6         & 7491.0          &  \textbf{4447.1}      \\
4 layers              & 5017.2           & 7503.8        & \textbf{4498.3}      \\
8 layers             &  5033.5        & 7764.5          & \textbf{4696.1}    \\
10 layers             & 4808.3       & 7697.4          & \textbf{4624.7}      \\
\hline
\end{tabular}
\caption{The cumulative regret of 10000 rounds on MovieLens with the different number of layers. }
\label{tablayer1}
\end{table}

\begin{table}[ht]
\centering
\begin{tabular}{c|cccccc|c}
\hline
               & NeuUCB-ONE         & NeuUCB-IND     & \sysn      \\ \hline
2 layers            & 6964.1         & 6911.7         &  \textbf{6773.4}      \\
4 layers            &  6944.7    &  6942.5       &  \textbf{6803.2}          \\
8 layers           & 7012.8    &     6932.2      &  \textbf{6878.3}    \\
10 layers             &6992.4      &    6987.4       &    \textbf{6854.9}         \\
\hline
\end{tabular}
\caption{The cumulative regret of 10000 rounds on Yelp with the different number of layers. }
\label{tablayer2}
\end{table}

\textit{Ablation Study for Network Layers}.
We run the experiments on MovieLens and Yelp datasets with the different number of layers of neural networks and report the results in Table \ref{tablayer1} and \ref{tablayer2}. \sysn achieves the best performance in most cases.
In this paper, we try to propose a generic framework to combine meta-learning and bandits with the neural network approximation. Since the UCB in \sysn only depends on the gradient, the neural network can be easily replaced by other different structures.

\iffalse
\begin{table}[ht]
	\vspace{1em}
	\centering
	\begin{tabular}{c|c|c|c}
		\toprule 
&  n = 5000 & n = 10000 & n = 20000  \\ 
	\toprule  
NeuUCB-One &  0.048  &   0.049 &    0.046   \\
NeuralLinear &  0.057 &  0.097 &  0.180    \\
NeuA+U &  0.053 &  0.054 &  0.058     \\
CLUB &   0.098  & 0.167 & 0.323 \\ 
\midrule  
M-CNB & 0.128 & 0.211 & 0.291 \\
\bottomrule
	\end{tabular}
 \caption{  Average running time of each method in one round }\label{tab:largenumber}
\end{table}

\textit{Running time}. As shown in Table \ref{tab:largenumber}, the running time of \sysn has the same magnitude as other baselines, because the cost of the two additional parts, Clustering and Meta training, are minor compared to user-learner training time.
The running time of M-CNB, NeuralLiner, and CLUB grows with the increasing number of users, because the clustering time of these three methods has increased linearly. But \sysn's running time still stays at the same magnitude compared to NeuralLiner and CLUB. 
Since NeuUCB-One and NeuA+U do not have the clustering procedure, their running time stays at the same magnitude.
This makes it feasible to implement \sysn to serve as a core component of the large recommender system.

\fi
